# Supplementary material for: Glassy dynamics in two-dimensional ring polymers: size versus stiffness polydispersity
Source: arXiv:2509.20066 source file (2025-09-24)
Supplement: Supplementary file 1 [file SuppInfo.pdf]

## Supplementary Material:

### Glassy dynamics in two-dimensional ring polymers: size versus stiffness polydispersity

Rahul Nayak,<sup>\*</sup> Pinaki Chaudhuri,<sup>†</sup> and Satyavani Vemparala<sup>‡</sup>

*The Institute of Mathematical Sciences, C.I.T. Campus, Taramani, Chennai 600113, India and  
Homi Bhabha National Institute, Training School Complex, Anushakti Nagar, Mumbai, 400094, India*

---

<sup>\*</sup> rahulnayak@imsc.res.in

<sup>†</sup> pinakic@imsc.res.in

<sup>‡</sup> vani@imsc.res.in

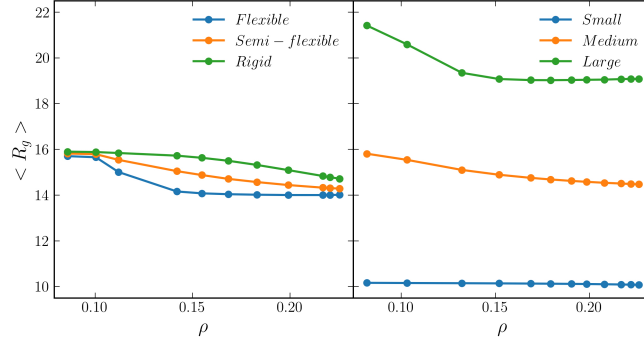

FIG. S1. Radius of gyration as a function of density for stiffness-polydisperse and size-polydisperse ring polymer systems.

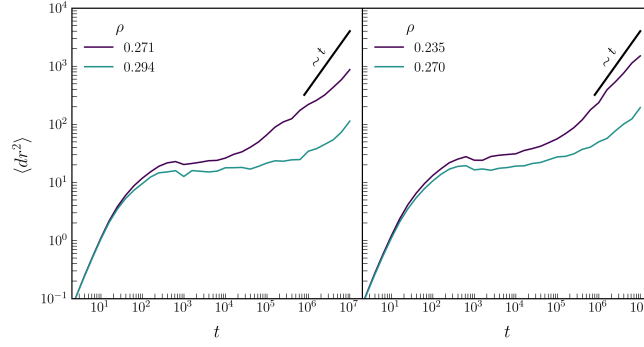

FIG. S2. MSD vs time plot for densities which fall in glassy regime in stiffness-polydisperse and size-polydisperse systems.

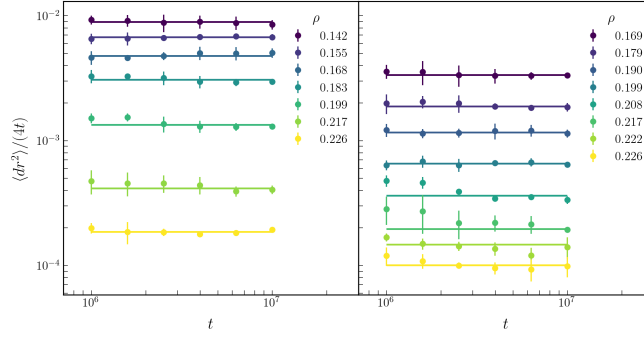

FIG. S3. Extraction of diffusion coefficient from the  $\langle dr^2 \rangle / 4t$  versus time in the long time regime for stiffness-polydisperse and size-polydisperse systems at various densities.

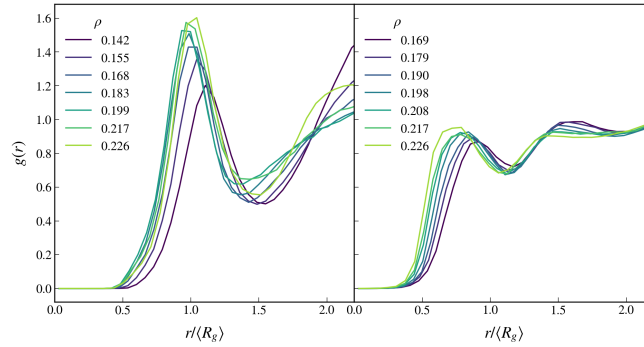

FIG. S4. Radial distribution function of stiffness-polydisperse and size-polydisperse ring polymer systems.
